# Supplementary material for: Streaming Diffusion Policy: Fast Policy Synthesis with Variable Noise Diffusion Models
Source: arXiv:2406.04806 source file (2024-10-11)
Supplement: Supplementary file 1 [file ImplementationDetails.tex]

\appendix
\section{Sampling with incomplete chunks in the buffer}
\label{app:implementation_notes}
As shown by \citet{chiDiffusionPolicyVisuomotor2023b}, values of $T_o$ and $T_a$ affect performance, and to do a fair comparison between the TEDi Policy and Diffusion Policy, we want to fix these parameters to $2$ and $8$, respectively. However, when fixing these parameters, there are no configurations possible if we respect both (i) the restriction that the input to the U-Net has to be divisible by 4 and (ii) we predict a multiple of $8$ actions into the future. Specifically, we would have to satisfy both 
$$T_p + (T_o - 1) \equiv 0 \pmod{T_a} \quad \text{and} \quad T_p \equiv 0 \pmod{4}.$$
Inserting $T_o=2$ and $T_a=8$, we get 
$$T_p + 1 \equiv 0 \pmod{8} \quad \text{and} \quad T_p \equiv 0 \pmod{4}$$
which does not have any solutions. Any number divisible by $4$ is either $\equiv 0$ or $\equiv 4 \bmod 8$. Therefore, we need to allow for values of $T_p-1$ that are not divisible by $T_a$, that is, we want to allow for \textit{incomplete chunks} in the buffer. To allow for this, we modify Algorithm \ref{alg:tedi_sampling} slightly. The changes are highlighted in \textcolor{blue}{blue}.

\begin{algorithm}
\caption{TEDi Policy Sampling}
\label{alg:tedi_sampling}
\begin{algorithmic}[1]
\REQUIRE Buffer $\mathbf{B}$, Denoiser $D_\theta(\rvx_\sigma, \sigma)$, Diffusion level per action $\mathbf{k}$, Observations $\mathbf{O}_t$
\IF{first step}
    \STATE $\mathbf{B}, \mathbf{k} \gets \text{Initialize buffer}(\mathbf{O}_t)$ 
\ENDIF
\WHILE{first chunk not clean} 
    \STATE $\mathbf{B}, \mathbf{k} \gets D_\phi(\mathbf{B}, \mathbf{O}_t, \mathbf{k})$ \hfill $\triangleright$ Denoise one step
\ENDWHILE 
\STATE $\mathbf{A}_t \gets \mathbf{B}[(T_o-1):T_o+T_a]$ \hfill $\triangleright$ Return first action sequence
\STATE $\mathbf{B} \gets \mathbf{B}[T_a:]$, $\mathbf{k} \gets \mathbf{k}[T_a:]$ \hfill $\triangleright$ Remove the first $T_a$ steps
\STATE \textcolor{blue}{$\mathbf{B} \gets \mathbf{B}[:-((T_p-(T_o-1))\text{\%} T_a)]$}
\STATE \textcolor{blue}{$\mathbf{k} \gets \mathbf{k}[:-((T_p-(T_o-1))\text{\%} T_a)]$ \hfill $\triangleright$ Remove the excess steps}
\STATE Sample $\mathbf{z} \sim \mathcal{N}(\mathbf{0}_{T_a \textcolor{blue}{+ ((Tp - (To - 1)) \text{\%} Ta)}}, \mathbf{I}_{T_a \textcolor{blue}{+ ((Tp - (To - 1)) \text{\%} Ta)}})$
\STATE $\mathbf{B}.\text{append}(\mathbf{z}), \mathbf{k}.\text{append}([N-1]_{\times T_a \textcolor{blue}{+ ((Tp - (To - 1)) \text{\%} Ta)}})$ \hfill $\triangleright$ Append $T_a$ steps of noise
\STATE $\mathbf{k}_\text{next} \gets \mathbf{k}[T_a]$ \hfill $\triangleright$ Get diffusion level for next chunk
\STATE add\_noise($\mathbf{B}[:(T_o-1)]$, $\mathbf{k}_\text{next}$) \hfill $\triangleright$ Noise clean actions overlapping with next observations
\RETURN $\mathbf{A}_t$
\end{algorithmic}
\end{algorithm}
